# Supplementary material for: The Limits of Transfer Reinforcement Learning with Latent Low-rank Structure
Source: arXiv:2410.21601 source file (2024-10-28)
Supplement: Supplementary file 1 [file lower_bound_proof.tex]

\section{Lower Bound Proofs} \label{app:lb_tr}
Before we present proof of Theorem \ref{thm:lb_tr}, we first present a lemma on hypothesis testing when the learner has access to a noisy oracle. 

\begin{lem}\label{lem:hyp}
Consider the problem of distinguishing between two Bernoulli distributions with mean $1/2, 1/2 - 1/\alpha$, and the learner is given a one-time use oracle that outputs the correct mean with probability $0.5 \leq \gamma \leq 0.775$. To identify the correct distribution with probability at least $0.975$, the learner still needs to observe $\Omega(\alpha^2)$ samples.
\end{lem}

Lemma \ref{lem:hyp} states having access to a noisy oracle does not improve the sample complexity lower bound on distinguishing between two similar Bernoulli distributions with high probability. This lemmas shows that if one cannot guarantee that the learned latent factor in the source problem is sufficient, then there is no benefit from transfer learning as learned knowledge from the source problem is effectively useless. See Appendix \ref{app:hyp} for the formal proof.

\subsection{Proof of Theorem \ref{thm:lb_tr}} 
We next prove Theorem \ref{thm:lb_tr}, which shows that one must incur a dependence on $\alpha$ to benefit from transfer learning. The proof follows the same steps as the proof of Theorem \ref{thm:lb_int} except we increase the size of the function class so that if the learner does not correctly identify the correct latent factor in the source MDPs, then the learner must find the optimal action at each state. 
\begin{proof}
Consider the construction where all source and target MDPs $(S, A, P, H, r)$ share the same state space, action space, and horizon $H = 1$ and assume that $S = A = [2n]$ for some $n \in \N_+$. For ease of notation, we let $s_1$ refer to any state in $[n]$ and $s_2$ refer to any state in $\{n+1, \ldots 2n\}$. Similarly, we let $a_1$ refer to the first half of the actions and let $a_2$ refer to the second half of the actions. The initial state distribution in the target MDP is uniform over $S$. In contrast to our intermediate lower bound, we consider a function class $\F$ of size $2^n$ where each state latent factor corresponds to a different sequence of $\sqrt{1/n}$ or $-\sqrt{1/n}$ in the first $n$ entries and zero in the second $n$ entries. Thus, $F \in \F$ has the following form 
\[
F_i(s) = \pm \sqrt{1/n} \text{ for } s \in [n], F_i(s) = 0 \text{ for } s \in \{n+1, \ldots 2n\},
\]
where the sequence of positives or negative values depends on $i$. Finally, we add a special state latent factor $F'$ to $\F$ that is orthogonal to all the previously specified latent factors $F_i$,
\[
F'(s_1) = 0, F'(s_2) = \sqrt{1/n}.
\]
We now present transfer RL problems with similar $Q$ functions (with rows $s_1, s_2$ and columns $a_1, a_2$) that satisfy Assumptions \ref{asm:tr} and \ref{asm:transfer}. For ease of notation, the superscript $i$ of $Q^{*, i}_{m, h}, Q^{*, i}_{ h}$ denotes the transfer RL problem.  Then, the optimal $Q$ functions for transfer RL problem $i$ are
\begin{align*}
    Q^{*, i}_{1, 1} &= n F_i G_1^\top = n \left[\begin{tabular}{c}
         $\pm \sqrt{1/n}$ \\
          $0$
    \end{tabular} \right] \left[\sqrt{1/n}, 0 \right] = \left[\begin{tabular}{cc}
         $\pm 1$ & 0  \\
         0 & 0
    \end{tabular} \right],   \\
    Q^{*, i}_{2, 1} &= n F_i G_2^\top =  n \left[\begin{tabular}{c}
         $\pm \sqrt{1/n}$ \\
          $0$
    \end{tabular} \right] \left[0, \sqrt{1/n} \right]=\left[\begin{tabular}{cc}
         0 & $\pm 1$  \\
         0 & 0
    \end{tabular} \right].
\end{align*}
In the target MDP, there exists one special action $a^*$ such that the target latent factor is $G_T(a^*) = \sqrt{1/(2n)}$ and $G_T(a) = -\sqrt{1/(2n)}$ for $a \in [2n], a \neq a^*$. The optimal $Q$ function in the target MDP of transfer RL problem $i$ is $Q^{*, i}_1 = n F_i G_T^\top$. Therefore, we have for $s \in [n]$,
\[
    Q^{*, i}_1(s, a) = \begin{cases}
        \sqrt{1/2} \text{ if } F_i(s) = \sqrt{1/n} \text{ and } a = a^*\\
        -\sqrt{1/2} \text{ if } F_i(s) = \sqrt{1/n} \text{ and } a \neq a^*\\
        \sqrt{1/2} \text{ if } F_i(s) = -\sqrt{1/n} \text{ and } a \neq a^*\\
        -\sqrt{1/2} \text{ if } F_i(s) = -\sqrt{1/n} \text{ and } a = a^*,
    \end{cases}
\]
and $Q^{*, i}_1(s, a) = 0 $ if $s \in \{n+1, \ldots, 2n\}$. Next, we define the optimal $Q$ functions for transfer RL problem $i'$. The $Q$ functions are
\begin{align*}
    Q^{*, i'}_{1, 1} &= n F_i G_1^\top = n \left[\begin{tabular}{c}
         $\pm \sqrt{1/n}$ \\
          $0$
    \end{tabular} \right] \left[\sqrt{1/n}, 0 \right] = \left[\begin{tabular}{cc}
         $\pm 1$ & 0  \\
         0 & 0
    \end{tabular} \right],   \\
    Q^{*, i'}_{2, 1} &= n F_i' G_2^\top =
    n \left[\begin{tabular}{c}
         $\pm \sqrt{1/n - 1/\beta^2}$ \\
          $1/\beta$
    \end{tabular} \right] \left[0, \sqrt{1/n} \right]
    = \left[\begin{tabular}{cc}
         0 & $\pm \sqrt{1 - n/\beta^2}$  \\
         0 & $\sqrt{n/\beta^2}$
    \end{tabular} \right]\\
    Q^{*, i'}_{1} & = n F'G_T^\top = \begin{cases}
        \sqrt{1/2} \text{ if } s \in \{n+1, \ldots, 2n\} \text{ and } a = a^*\\
        -\sqrt{1/2} \text{ if } s \in \{n+1, \ldots, 2n\} \text{ and } a \neq a^*\\
        0 \text{ if } s \in [n].
    \end{cases}
\end{align*}
Thus, in transfer RL problems $i$ and $i'$, in the target phase, one should choose action $a^*$ or any other action at state $s$ depending on $F(s)$. Note that the incoherence $\mu$, rank $d$, and condition number $\kappa$ in each of the above $Q$ functions are all $O(1)$. Clearly, the above construction satisfies Assumption \ref{asm:tr} with Tucker rank $(|S|, 1, |A|)$. Furthermore, both transfer learning problems satisfy Assumption \ref{asm:transfer} because 
\[
F' = -\sqrt{\beta^2/n - 1}F_i + \sqrt{\frac{\beta^2 }{n}} F_i',
\]
and it follows that $\alpha= \sqrt{\beta^2/n}$.

First, $i$ is sampled uniformaly from the set $[2^n]$, and the learner is given transfer RL problem $i$ or $i'$ with equal probability with a generative model in the source problem. When interacting with the source MDPs, the learner specifies a state-action pair $(s, a)$ and source MDP $m$ and observes a realization of a shifted and scaled Bernoulli random variable $X$. The distribution of $X$ is that $X = 1$ with probability $(Q^{*, i}_{m, 1}(s, a) + 1)/2$ and $X = -1$ with probability $(1 - Q^{*, i}_{m, 1}(s, a))/2)$. Furthermore, the learner is given the knowledge that  the state latent features lies in the function class $\F$ but is not told the value $i$ and must use the knowledge in the source MDP to guess which latent factor to use in the target MDP. Giving the learner the function class is no harder than the same problem without receiving this additional information. In contrast to the setting of our intermediate lower bound, we allow the learner to switch that latent factor they use in the target phase. Note that in this construction, the sub-optimality gap $\Delta_{\min} = \sqrt{2}$; by changing $\sigma$, we can decrease $\Delta_{\min}$. 

We first note that $\| Q^{*, i'}_{2, 1} -  Q^{*, i}_{2, 1}\|_\infty \leq \sqrt{n/\beta^2} = 1/\alpha$. Then, from \cite{Anthony_Bartlett_1999}, there exists a constant $C$ such that if the learner observes $n$ samples in the source MDPs at one specific state-action pair $(s_2, a_2)$, where $n \leq C\alpha^2$, then the probability of the learner correctly identifying the correct latent factor $F_i$ or $F_i'$ is upper bounded by $0.76$. 

To learn an optimal policy, one must correctly identify the feature representation as one needs to determine whether to take action $a^*$ or any other action at each state (depending on whether $F_i(s) = \sqrt{1/n} \text{ or } -\sqrt{1/n}$. To correctly identify $a^*$, one needs to observe at least $\Omega(|A|/\Delta_{\min}^2)$ samples with probability at least $0.9$ \cite{wang2020statistical}. 

Then, using the guess on the latent factor as our noisy oracle, Lemma \ref{lem:hyp} states that to correctly identify whether to choose action 0 or action $a^*$ at each state (distinguishing between two Bernoulli distributions) one needs $\Omega(|S|/\Delta_{\min}^2)$ samples.

Finally, taking a union bound gives us the desired result; to learn an optimal policy, one needs to observe $\Omega(\alpha^2)$ samples in the source MDP or $\Omega((|S| + |A|)/\Delta_{\min}^2)$ episodes in the target MDP where $\Delta_{\min} = \sqrt{2}$ with probability at least $0.875$.

\end{proof}

\subsection{Proof of Theorem \ref{thm:lb_lr}} \label{app:lb_lr}
In this section, we present the proof of Theorem \ref{thm:lb_lr}. The proof is similar to the proof of Theorem \ref{thm:lb_tr} but accounts for the different Tucker rank setting.
\begin{proof}
Consider the construction where all source and target MDPs $(S, A, P, H, r)$ share the same state space, action space, and horizon with $M = 2$. Assume that $S = A = [2n]$ for some $n \in \N_+$. For ease of notation, we let $s_1$ refer to any state in $[n]$ and $s_2$ refer to any state in $\{n+1, \ldots 2n\}$. Similarly, we let $a_1$ refer to the first half of the actions and let $a_2$ refer to the second half of the actions. The initial state distribution in the target MDP is uniform over $S$. 

We consider two transfer RL problems, in which the source MDPs have similar transition kernels but differing $\phi$. Let the feature mapping for transfer RL problem $i$ be $\phi_i \in \Phi$. Let the superscript of the transition kernel denote the transfer RL problem. For $\beta> 0$, the transition kernels for the transfer RL problem  $i$  are 
\begin{align*}
    P_{1, h}^i(s_1|\cdot, \cdot) &= \mu_{1, h}(s_1) \phi_{i, h}(\cdot, \cdot)^\top = \left[\frac{1}{2n}, \frac{1}{2n} + \frac{1}{n\beta} \right] \phi_{i, h}(\cdot, \cdot)^\top ,\\
    P_{1, h}^i(s_2|\cdot, \cdot) &=   \mu_{1, h}(s_2) \phi_{i, h}(\cdot, \cdot)^\top = \left[\frac{1}{2n}, \frac{1}{2n} - \frac{1}{n\beta} \right] \phi_{i, h}(\cdot, \cdot), \\
    P_{2, h}^i(\cdot| \cdot, \cdot) &= \mu_{2, h}(\cdot) \phi_{i, h}(\cdot, \cdot)^\top = \left[\frac{1}{2n}, \frac{1}{2n}\right] \phi_{i, h}(\cdot, \cdot) = \frac{1}{2n}, \\
    P_{h}^i(\cdot| \cdot, \cdot) &= \mu_{h}(\cdot) \phi_{i, h}(\cdot, \cdot)^\top = \left[\frac{1}{2n}, \frac{1}{2n}\right] \phi_{i, h}(\cdot, \cdot) = \frac{1}{2n}, \\
    P_{H-1}^i (s_1 |\cdot, \cdot) &= \mu_{H-1}(s_1) \phi_{i, H-1}(\cdot, \cdot)^\top = \left[\frac{1}{2n}, \frac{3}{4n} \right]\phi_{i, h}(\cdot, \cdot)\\
    P_{H-1}^i (s_2 |\cdot, \cdot) &= \mu_{H-1}(s_2) \phi_{i, H-1}(\cdot, \cdot)^\top = \left[\frac{1}{2n}, \frac{1}{4n} \right]\phi_{i, h}(\cdot, \cdot).
\end{align*}
Since $\mu_{T, H-1}(s_1) = \frac{\beta}{4} \mu_{1, H-1}^i(s_1) + (1 - \frac{\beta}{4})\mu_{2, H-1}^i $ for both $i$, it is clear that the construction is a Low Rank MDP and satisfies Assumption \ref{asm:task} with $\alpha = \beta/4$. Let $f_a: S \to A$. Then, the feature mapping $\phi^{f_a, x}$ has the form 
\[
\phi^{f_a, x}(s, f_a(s)) = [0, 1]^\top, \phi^{f_a, x}(s, a) = [ 1-x, x]^\top
\]
for $a \neq f_a(s)$ and $x \in \{0, 0.25\}$. Let $F_a$ be set of all $|A|^{|S|}$ mappings $f_a$. Then, our function class is $\Phi = \{ \phi^{f, x}| f \in F_a, x \in \{0, 0.25\} \}$. It follows that $|\Phi| = 2^{|A|^{|S|}}$. With $\phi_1, \phi_2 \in \Phi$ for $\phi_1 \neq \phi_2$, it follows that the entries from transition kernel from transfer RL problem $1$ and problem $2$ differ by at most $1/(n\beta)$. 
 
Next, for $\eps > 0$, the reward functions in the target MDP for transfer RL problem $i$ are 
\begin{align*}
r_h(\cdot, \cdot) &= [1/2 - \eps, 1/2] \phi_i(\cdot, \cdot) \text{ for } h < H\\
r_H(\cdot, \cdot) &= [0, 0] \phi_i(\cdot, \cdot).
\end{align*}

Then, the learner is given transfer RL problem $i$ or transfer RL problem $j$ with equal probability where the unique optimal action at each state and time step differs between $\phi_i$ and $\phi_j$. The learner is given a generative model in the source problem where the learner can observe samples from the transition kernels. Querying the generative model takes in a state-action pair $(s, a)$ and returns a next state $s'$ given by a realization of $P_{m, h}^i(\cdot|s, a)$. Furthermore, the learner is given $\phi_1$ and $\Phi$ and must use the knowledge in the source MDPs to discern which one to use in the target MDP, which is no harder than the same problem without the extra information.

We first note that there exists a constant $C$ such that if the learner observes $n$ samples in the source MDPs at one specific state-action pair, where $n \leq C\alpha^2$, then the probability of the learner correctly identifying the $\phi$ is upperbounded by $0.76$ \cite{Anthony_Bartlett_1999}. 

Since the instantaneous regret of choosing any sub-optimal action is $3\eps/4$ at any time step (excluding time step $H$), one needs to correctly identify $\phi$ to learn an $\eps/4$ optimal policy. 
 As the occupancy distribution of every policy at each time step is uniform (as the transition kernel in all target MDPs is the uniform transition kernel), one must identify the correct feature representation (or optimal action) at each state to guarantee the policy is $\eps/4$-optimal.

 Using the estimated $\phi$ as the oracle, Lemma \ref{lem:hyp} states that one needs $\Omega(1/\eps^2)$ samples to identify the optimal action when comparing two actions (two Bernoullis with different means) at each state with high probability. Since one needs to try $\Omega(A)$ actions to guarantee that one finds the optimal action, $\Tilde{\Omega}(|A|/\eps^2)$ samples are needed at each state and each time step. 
Finally, a union bound gives us the desired result; to learn an $\eps/4$-optimal policy, one needs to observe $\Omega(\alpha^2)$ samples in the source MDP or $\Tilde{\Omega}(|S||A|H/\eps^2)$ episodes in the with probability at least $0.875$.
\end{proof}

\subsection{Hypothesis Testing with a Noisy Oracle}\label{app:hyp}
In this section, we prove Lemma \ref{lem:hyp}.
\begin{proof}
We assume the setting of Lemma \ref{lem:hyp}. For ease of notation, we let the oracle be a Bernoulli distribution where 1 refers to the distribution with mean $1/2$ and 0 refers to the distribution with mean $1/2 - 1/\alpha$. Now, assume that the learner observes $n$ samples of the distribution $\{X_i\}_{i \in [n]}$. We denote $P_0$ as the setting, in which the true mean is $p = 1/2$ which implies that the distribution of the oracle is $Bern(\gamma)$, and denote $P_1$ as the setting, in which the true mean is $1/2 - 1/\alpha$ which implies that the distribution of the oracle is $Bern(1-\gamma)$ as zero corresponds to the mean of $1/2 - 1/\alpha$. Let $\Psi$ be the set containing all decision rules that map $\{X_i\}_{i \in [n]} \to \{0, 1\}$. Then, from Le Cam's method \cite{lecam}, we have that error rate, i.e., the probability that the best decision rule the learner can use is wrong, is equal to 
\[
P(E) = \inf_{\psi \in \Psi} \left(P_0(\psi(\{X_i\}_{i \in [n]})  =  1) +  P_1(\psi(\{X_i\}_{i \in [n]})  =  0)       \right) =  1 - \|P_0 - P_1\|_{TV},
\]
where $E$ is the event that the best decision rule the learner can use is wrong. Then, from Pinsker's lemma and the fact that the KL divergence between product distributions is the sum of the KL divergence of the individual distributions, we have that 
\[
P(E) = 1 - \|P_0 - P_1\|_{TV} \geq 1 - \sqrt{\frac{n D_{KL}(Bern(1/2)\|Bern(1/2 - 1/\alpha)) + D_{KL}(Bern(\gamma)\|Bern(1- \gamma) )}{2}}
\]
Since $\log(x) \leq x -1 $ for $x \geq 0$, it follows that the KL Divergence between two Bernoulli distributions with parameters $u, v$ satisfy
\[
D_{KL}(u\|v) = u \log(u/v) + (1-u)\log((1-u)/(1-v)) \leq \frac{(u-v)^2}{v(1-v)}.
\]
Clearly, $D_{KL}(Bern(\gamma)\|Bern(1- \gamma))=  \frac{(2\gamma-1)^2}{\gamma(1-\gamma)}$ is maximized when $\gamma = 0.775$ for $\gamma \in [0.5, 0.775]$, so 
\[
D_{KL}(Bern(\gamma)\|Bern(1- \gamma)) \leq 1.73477.
\]
It follows that 
\begin{align*}
P(E) &\geq 1 - \sqrt{\frac{n D_{KL}(Bern(1/2)\|Bern(1/2 - 1/\alpha)) + D_{KL}(Bern(\gamma)\|Bern(1- \gamma) )}{2}} \\
&\geq 1 - \sqrt{\frac{8n/\alpha^2 + 1.73477 }{2}}.
\end{align*}
Solving $1 - \sqrt{\frac{8n/\alpha^2 + 1.73477 }{2}} \geq 0.125$ for $n$ gives
\[
P(E) \geq 0.125
\]
for $n \leq C \alpha^2$ for some absolute constant $C > 0$, which implies that the learner identifies the correct distribution with probability at most $0.975$. 
\end{proof}
