# Supplementary material for: The Limits of Transfer Reinforcement Learning with Latent Low-rank Structure
Source: arXiv:2410.21601 source file (2024-10-28)
Supplement: Supplementary file 2 [file tucker_rank_ssd.tex]

\section{$(\cardS , \cardS , d)$ Tucker Rank Setting}\label{app:tr_ssd}
In this section, we present the assumptions, algorithm, and results for the $(\cardS , \cardS , d)$ Tucker rank setting. In this setting, we assume the following structure on the source and target MDPs.
\begin{assumption}\label{asm:tr_s}
In each of the $M$ source MDPs and in the target MDP, the reward functions have rank $d$, and the transition kernels have Tucker rank $(\cardS , \cardS , d)$. Thus, there exists $\cardS  \times \cardS  \times d$ tensors $U_{m, h}, U_h$ s, $\cardA  \times d$ orthonormal matrices $G_{m, h}, G_h$, and $\cardS  \times d$ matrices $W_{m, h}, W_{ h}$ such that 
\begin{align*}
P_{m, h}(s'|s, a) &= \textstyle\sum_{i \in [d]} G_{m, h}(a, i)U_{m, h}(s',s, i) , \\
r_{m, h}(s, a)
&= \textstyle\sum_{i \in [d]} G_{m, h}(a, i) W_{m, h}(s, i)
\end{align*}
and 
\begin{align*}
P_{h}(s'|s, a) &= \textstyle\sum_{i \in [d]} G_h(s, i)U_h(s', s, i) ,\\
r_{ h}(s, a)
&= \textstyle\sum_{i \in [d]} G_h(s, i) W_{ h}(s, i)
\end{align*}
where $\|\sum_{s' \in S} g(s') U_{m, h}(s', s, :)\|_2$,$ \|\sum_{s' \in S}g(s') U_{ h}(s', s,:)\|_2, \|W_{h}(s)\|_2, \|W_{m, h}(s)\|_2 \leq \sqrt{\cardA /(d\mu)}$ for all  $s \in S$, $a \in A$, $h\in[H]$, and $m\in [M]$ for any function $g:S \to [0, 1]$. 
\end{assumption}

Similarly, to allow transfer of a latent representation between the source and target MDPs, we assume that the subspace spanned by the set of all source latent factors contains the space spanned by the set of target latent factors.

\begin{assumption}\label{asm:transfer_s}
Suppose Assumption \ref{asm:tr_s} holds. For latent factors $G_h$ from the target MDP and $G_{m, h}$ for the source MDPs, let $G_h = \{G_h, G_{h, m}\}_{m\in [M]}$. Then, there exists a non-empty set $\B(G_h)$ such that the elements in $\B(G_h)$ are $B_h \in \R^{d, d, M}$ such that 
\[
G_h(s, i) = \textstyle\sum_{j \in [d], m \in [M]} B_h(i, j, m) G_{m, h}(s, j)
\]
for all $i \in [d], s \in \cS, h \in [H]$.
\end{assumption}
The transfer-ability coefficient in this setting quantifies the efficacy of transfer learning. 

\begin{definition}\label{def:tc_s}
Given a transfer RL problem that satisfies Assumptions~\ref{asm:tr_s}, \ref{asm:transfer_s}, and \ref{asm:full_rank}, let $\mathcal{G}$ be the set of all $\R^{\cardA  \times d}$ orthonormal latent factor matrices with columns that span the column space of $Q^*_{m, h}$ for all $m \in [M], h \in [H]$. Then, we define $\alpha$ as 
\[
\alpha \coloneqq \min_{G \in \mathcal{G}}\min_{B \in \B(G)} \max_{i, j \in [d], m\in [M]} |B(i, j, m)|.
\]
\end{definition}

We now prove our lower bound in this Tucker rank setting that states that one must incur a source sample complexity of $\Omega(\alpha^2)$ to benefit from transfer learning. 
\begin{thm}\label{thm:lb_ssd}
    Let $\F$ be a function class containing the true latent feature representation.
    There exists a transfer RL instance that satisfies Assumptions \ref{asm:tr_s} and \ref{asm:transfer_s} in which the only information the learner can transfer between the source and target phases is a latent feature representation in $\F$. Then, to learn an optimal policy in the target MDP, the learner needs to incur a sample complexity of $\Omega(\alpha^2)$ in the source MDP or $\Omega((\cardS  + \cardA )/\Delta_{\min}^2)$ in the target MDP with probability at least $0.4375$.
\end{thm}

The proof of Theorem \ref{thm:lb_ssd} follows the same construction used to prove Theorem \ref{thm:lb_tr} except we swap the state and action latent factors. 
\begin{proof}
Consider the construction where all source and target MDPs $(\cS, \cA, P, H, r)$ share the same state space, action space, and horizon $H = 1$ and assume that $\cS = \cA = [2n]$ for some $n \in \N_+$. For ease of notation, we let $s_1$ refer to any state in $[n]$ and $s_2$ refer to any state in $\{n+1, \ldots 2n\}$. Similarly, we let $a_1$ refer to the first half of the actions and let $a_2$ refer to the second half of the actions. The initial state distribution in the target MDP is uniform over $\cS$. We consider a function class $\F$ of size $2^n$ where each state latent factor corresponds to a different sequence of $\sqrt{1/n}$ or $-\sqrt{1/n}$ in the first $n$ entries and zero in the second $n$ entries. Thus, $G \in \F$ has the following form 
\[
G_i(a) = \pm \sqrt{1/n} \text{ for } a \in [n], G_i(a) = 0 \text{ for } a \in \{n+1, \ldots 2n\},
\]
where the sequence of positives or negative values depends on $i$. Finally, we add a special state latent factor $G'$ to $\F$ that is orthogonal to all the previously specified latent factors $G_i$,
\[
G'(s_1) = 0, G'(s_2) = \sqrt{1/n}.
\]
We now present transfer RL problems with similar $Q$ functions (with rows $s_1, s_2$ and columns $a_1, a_2$) that satisfy Assumptions \ref{asm:tr_s} and \ref{asm:transfer_s}. For ease of notation, the superscript $i$ of $Q^{*, i}_{m, h}, Q^{*, i}_{ h}$ denotes the transfer RL problem.  Then, the optimal $Q$ functions for transfer RL problem $i$ are
\begin{align*}
    Q^{*, i}_{1, 1} &= n F_1 G_i^\top = n \left[\begin{tabular}{c}
         $ \sqrt{1/n}$ \\
          $0$
    \end{tabular} \right] \left[\pm\sqrt{1/n}, 0 \right] = \left[\begin{tabular}{cc}
         $\pm 1$ & 0  \\
         0 & 0
    \end{tabular} \right],   \\
    Q^{*, i}_{2, 1} &= n F_2 G_i^\top =  n \left[\begin{tabular}{c}
         $0$ \\
          $\sqrt{1/n}$
    \end{tabular} \right] \left[\pm \sqrt{1/n}, 0 \right]=\left[\begin{tabular}{cc}
         0 & $0$  \\
         $\pm 1$ & 0
    \end{tabular} \right].
\end{align*}
In the target MDP, there exists one special state $s$ such that the target latent factor is $F_T(s^*) = \sqrt{1/(2n)}$ and $F_T(s) = -\sqrt{1/(2n)}$ for $s \in [2n], s \neq s^*$. The optimal $Q$ function in the target MDP of transfer RL problem $i$ is $Q^{*, i}_1 = n F_T G_i^\top$. Therefore, we have for $s \in [n]$,
\[
    Q^{*, i}_1(s, a) = \begin{cases}
        \sqrt{1/2} \text{ if } G_i(a) = \sqrt{1/n} \text{ and } s = s^*\\
        -\sqrt{1/2} \text{ if } G_i(a) = \sqrt{1/n} \text{ and } s \neq s^*\\
        \sqrt{1/2} \text{ if } G_i(a) = -\sqrt{1/n} \text{ and } s \neq s^*\\
        -\sqrt{1/2} \text{ if } G_i(a) = -\sqrt{1/n} \text{ and } s = s^*,
    \end{cases}
\]
and $Q^{*, i}_1(s, a) = 0 $ if $a \in \{n+1, \ldots, 2n\}$. Next, we define the optimal $Q$ functions for transfer RL problem $i'$. The $Q$ functions are
\begin{align*}
    Q^{*, i'}_{1, 1} &= n F_1 G_i^\top = n \left[\begin{tabular}{c}
         $\sqrt{1/n}$ \\
          $0$
    \end{tabular} \right] \left[\pm \sqrt{1/n}, 0 \right] = \left[\begin{tabular}{cc}
         $\pm 1$ & 0  \\
         0 & 0
    \end{tabular} \right],   \\
    Q^{*, i'}_{2, 1} &= n F_2 G_i'^\top =
    n \left[\begin{tabular}{c}
         0\\
         $\sqrt{1/n}$
    \end{tabular} \right]  \left[ \pm \sqrt{1/n - 1/\beta^2}, \pm 1/\beta \right]
    = \left[\begin{tabular}{cc}
         0 & 0  \\
         $\pm \sqrt{1 - n/\beta^2}$ & $ \pm \sqrt{n/\beta^2}$
    \end{tabular} \right]\\
    Q^{*, i'}_{1} & = n F_TG_{T, i}^\top = \begin{cases}
        \sqrt{1/2} \text{ if } a = a^* \text{ and } s = s^*\\
        -\sqrt{1/2} \text{ if } a \in \{n+1, \ldots, 2n\}, a \neq s^* \text{ and } s \neq s^*\\
        0 \text{ if } s \in [n],
    \end{cases}
\end{align*}
where for each $i$, there exists one unique action in $\{n +1, \ldots, 2n\}$ such that $G_i'(a^*) = 1/\beta$; let the unique action be $\lceil n + \log_2(i) \rceil$. For every other action $a \in \{n+1, \ldots, 2n\}, a \neq a^*$, we have $G_i'(a) = -1/\beta$. Similarly, $G_{T, i} = [0, \pm \sqrt{1/n}]$, where $G_{T, i}$ is only positive when the chosen action is $a^*$.
Thus, in transfer RL problems $i$ and $i'$, in the target phase, the optimal action depends on whether the current state is the special state $s'$. Note that the incoherence $\mu$, rank $d$, and condition number $\kappa$ in each of the above $Q$ functions are all $O(1)$. Clearly, the above construction satisfies Assumption \ref{asm:tr_s} with Tucker rank $(\cardS , \cardS , d)$. Furthermore, both transfer learning problems satisfy Assumption \ref{asm:transfer_s} because 
\[
G_{T, i} = -\sqrt{\beta^2/n - 1}G_i + \sqrt{\frac{\beta^2 }{n}} G_i',
\]
and it follows that $\alpha= \sqrt{\beta^2/n}$.

First, $i$ is sampled uniformaly from the set $[2^n]$, and the learner is given transfer RL problem $i$ or $i'$ with equal probability with a generative model in the source problem. When interacting with the source MDPs, the learner specifies a state-action pair $(s, a)$ and source MDP $m$ and observes a realization of a shifted and scaled Bernoulli random variable  $X_{s, a}$. The distribution of $X_{s, a}$ is that $X_{s, a} = 1$ with probability $(Q^{*, i}_{m, 1}(s, a) + 1)/2$ and $X_{s, a} = -1$. Furthermore, the learner is given the knowledge that the action latent features lies in the function class $\F$ but is not told the value $i$ and must use the knowledge in the source MDP to guess which latent factor to use in the target MDP. Giving the learner the function class is no harder than the same problem without receiving this additional information. We allow the learner to switch that latent factor they use in the target phase. Note that in this construction, the sub-optimality gap is $\Delta_{\min} = \sqrt{2}$; by changing $\sigma$, we can decrease $\Delta_{\min}$. 

We first note that $\| Q^{*, i'}_{2, 1} -  Q^{*, i}_{2, 1}\|_\infty \leq \sqrt{n/\beta^2} = 1/\alpha$. Then, from \cite{Anthony_Bartlett_1999},   if the learner observes $Z$ samples in the source MDPs at one specific state-action pair $(s_2, a_2)$, where $Z \leq O(\alpha^2)$, then the probability of the learner correctly identifying the correct latent factor $G_i$ or $G_i'$ is upper bounded by $0.76$. 

With $50\%$ chance, the learner is given the second transfer RL problem. To learn an optimal policy, one must correctly identify the feature representation as one needs to determine which action to take at state $s*$ and every other state. To correctly identify the special state, one needs to observe at least $\Omega(\cardS /\Delta_{\min}^2)$ samples with probability at least $0.9$ \cite{wang2020statistical}. 

Then, using the guess on the latent factor as our noisy oracle, Lemma \ref{lem:hyp} states that to correctly identify action $a^*$ as one needs to play $a^*$ at state $s^*$ (distinguishing between two Bernoulli distributions) one needs $\Omega(\cardA /\Delta_{\min}^2)$ samples. 

Finally, taking a union bound gives us the desired result;, to learn an optimal policy, one needs to observe $\Omega(\alpha^2)$ samples in the source MDP or $\Omega((\cardS  + \cardA )/\Delta_{\min}^2)$ episodes in the target MDP where $\Delta_{\min} = \sqrt{2}$ with probability at least $0.4375$. 
\end{proof}

Our algorithm in this setting is essentially the same as the algorithm used in the $(\cardS , d, \cardA )$ Tucker rank setting except we construct our latent factors using the other set of singular vectors. Furthermore, we compute Gram matrices and coefficients for each state instead of each action.

\begin{algorithm}
\caption{Source Phase}\label{alg:src_ssd}
\begin{algorithmic}[1]
\Require $\{N_h\}_{h \in [H]}$
\For{ $m \in [M]$}
\State Run LR-EVI($\{N_h\}_{h \in [H]})$ on source MDP $m$ to obtain $\bar{Q}_{m, h}$.
\State Compute the singular value decomposition of $\bar{Q}_{m, h} = \hat{F}_{m, h} \hat{\Sigma}_{m, h} \hat{G}_{m,h}^\top$ .
\EndFor
\State Compute feature mapping $\Tilde{G} = \{\Tilde{G}_h \}_{h \in [H]}$ with
$
\Tilde{G}_h  = \left \{ \sqrt{\frac{\cardA }{d\mu}}\hat{G}_{m, h}(:, i)|i \in [d],  m \in [M] \right\}.$
\end{algorithmic}
\end{algorithm}

\begin{algorithm}
\caption{Target Phase: LSVI-UCB-(S, S, d)}\label{alg:target_s}
\begin{algorithmic}[1]
\Require $\lambda, \beta_{k, h}^s, \Tilde{G} $
\For{ $k \in [K]$}
\State Receive initial state $s_1^k$.
\For {$h = H, \ldots, 1$}
\For {$s \in S$}
\State Set $\Lambda_h^s \xleftarrow{} \sum_{t \in T_{k-1, h}^s} \Tilde{G}_h(a_h^t)\Tilde{G}_h(a_h^t)^\top+ \lambda \textbf{I}$.
\State Set $w_h^s \xleftarrow{} (\Lambda_h^s)^{-1} \sum_{t \in T_{k-1, h}^s} \Tilde{G}_h(a_h^t)$ $\Big[r_h(s, a_h^t)+ \max_{a' \in A} Q_{h+1}(s_{h+1}^t, a') \Big]$.
\EndFor
\State Set $Q_h(\cdot, \cdot) \xleftarrow[]{} \min\Big(H, \langle w_h^\cdot, \Tilde{G}_h(\cdot)\rangle + \beta_{k, h}^\cdot \sqrt{ \Tilde{G}_h(\cdot)^\top (\Lambda_h^\cdot)^{-1} \Tilde{G}_h(\cdot)}\Big)  $.
\EndFor
\For{$h \in [H]$}
\State Take action $a_h^k \xleftarrow[]{} \max_{a \in A} Q_h(s_h^k, a), $ and observe $s_{h+1}^k$.
\EndFor
\EndFor
\end{algorithmic}
\end{algorithm}

We first present the theoretical guarantees of LSVI-UCB-(S, S, d) and defer their proofs to Appendix \ref{app:alg_proof}.  
\begin{thm}\label{thm:reg_s}
    Assume that Assumption \ref{asm:tr_s} holds and the learner is given the true latent action representation $G = \{G_h\}_{h \in [H]}$. Then, there exists a constant $c > 0$ such that for any $\delta \in (0, 1)$, if we set $\lambda = 1, \beta_{k, h}^s= c dH\sqrt{\iota}, \iota = \log(2dT\cardS /\delta)$, then with probability at least $1 - \delta$, the total regret of Algorithm \ref{alg:target_s} is $\Tilde{O}(\sqrt{d^3\cardS H^3T})$.
\end{thm}
Theorem \ref{thm:reg_s} states that LSVI-UCB-(S, S, d) completely removes the regret bound's dependence on the size of the state space by utilizing the latent action representation $G$. Similarly, the algorithm is robust to misspecification error.  
\begin{assumption}[$\xi$-approximate $(\cardS , \cardS , d)$ Tucker rank MDP]\label{asm:miss_s}
Assume $\xi \in [0, 1]$. Then, an MDP $(\cS, \cA, P, r, H)$ is a $\xi$-approximate $(\cardS , \cardS , d)$ Tucker rank MDP with given feature map $G$ if there exist $H$ unknown $\cardS $-by-$d$ matrices $W = \{W_h\}_{h \in [H]}$ and $\cardS$-by-$\cardS $-by-$d$ tensors $U = \{U_h\}_{h \in [H]}$ such that
\[
|r_h(s,a ) - W_h(s)^\top G_h(a)| \leq \xi,\]
\[\|P_h(\cdot|s, a) -  U_h(\cdot, s)G_h(a)^\top\|_{TV} \leq \xi
\]
for all $h \in [H]$ where $\|W_h\|_2, \|\sum_{s' \in S} g(s')U_h(s', a)\|_2 \leq \sqrt{\cardA /(d\mu)}$ for any function $g: \cS \to [0, 1]$.
\end{assumption}
\begin{thm}\label{thm:miss_s}
Under the Assumption \ref{asm:miss_s}, for any $\delta \in (0, 1)$, for $\lambda = 1, \beta_{k, h}^s = O(Hd\sqrt{\iota} + \xi\sqrt{kd}H)$ for $\iota =\log(2dT\cardS /\delta)$, the regret of Algorithm \ref{alg:target_s} is $\Tilde{O}(\sqrt{d^3H^3\cardS T} + \xi dHT)$ with probability at least $1 - \delta$.
\end{thm}

Next, we present and prove our main result in this setting (Theorem \ref{thm:tl_ssd}).

\begin{thm}\label{thm:tl_ssd}
Suppose Assumptions \ref{asm:tr}, \ref{asm:transfer}, and \ref{asm:full_rank} hold in the $(\cardS , \cardS , d)$ Tucker Rank setting, and set $\delta \in (0, 1)$. Furthermore, assume that for any $\eps \in (0, \sqrt{\cardS H/T})$,  $Q_{m, h} = r_{m, h} + P_{m, h} V_{m, h+1}$ has rank $d$ and is $\mu$-incoherent with condition number $\kappa$ for all $\eps$-optimal value functions $V_{h+1}$. Then, $T \geq  \frac{\cardS }{ \alpha^2}$, using at most 
\[
\Tilde{O} \left( d^4 \mu^4\kappa^4(1+\cardA /\cardS )M^2  H^4\alpha^2  T \right) 
\]
samples in the source problems, our algorithm has regret at most
\[
\Tilde{O}\left( \sqrt{(dMH)^3 \cardS T}\right)
\]
with probability at least $1 - \delta$ for $\lambda = 1$ and $\beta_{h, k}^s$, which is a function of $d, H, |T_{h, k}^s|, |S|, T, M$.  
\end{thm}
\begin{proof}
Suppose the assumption stated in Theorem \ref{thm:tl_ssd} hold. Then, from \cite{sam2023overcoming}, running LR-EVI with a sample complexity of    $C' d^4 \mu^4\kappa^4(\cardS +\cardA )M  H^4\alpha^2  T\log(2\cardS \cardA d MH/\delta)/ \cardS $ on each source MDP results in $\bar{Q}_{m, h}$ functions with singular value decomposition $\bar{Q}_{m, h} = \hat{F}_{m, h} \hat{\Sigma}_{m, h} \hat{G}_{m, h}$ that are $ \sqrt{H \cardS }/(2\alpha  \mu \kappa   \sqrt{d M T })$-optimal with probability at least $1 - \delta/2$.

Since our estimates are $\sqrt{H\cardS }/(2\alpha  \mu  \sqrt{d M T })$-optimal, it follows that $\bar{\gamma} < 1/2$ in the singular vector perturbation bound, Corollary \ref{cor:sv}. Since $\|Q^*_{m, h}\|_\infty \geq C$, from Corollary \ref{cor:sv}, it follows that there exists rotation matrices $R_{m, h}$ such that 
\[
\| (\hat{G}_{m, h} R_{m, h} - G_{m, h})(a)\|_{2} \leq \frac{d\sqrt{H  \mu \cardS }}{\alpha \sqrt{\cardA  M T}}
\]
for all $a \in A$ where the optimal $Q$ function have singular value decomposition $Q^*_{m, h} = F_{m, h}\Sigma_{m, h} G_{m, h}^\top$. 
 
Let $\Tilde{G}$ be the $\cardA  \times dM$ matrix from joining all the source action latent factor matrices, and $\hat{\Tilde{G}}_h$ be the $\cardA  \times dM$ matrix from joining all $\bar{G}_{m, h}$. Let $R_h$ be the $d \times dM$ matrix that joins $R_{m, h}$ for all $m \in [M]$. Then, from Assumption \ref{asm:transfer_s} and Definition \ref{def:tc_s}, it follows that for all $(s', s, a) \in \cS\times \cS\times A$, that 
\begin{align*}
    r_h(s, a) &= \sum_{i \in [d]} W_h(s, i)G_h(a, i) \\
    &= \sum_{i \in [d]} \left(\sum_{j \in [d], m \in [M]} B(i, j, m)G_{h, m}(a, j) \right)W_h(s, i)\\
    &= \sum_{i, j \in [d], m \in [M]} B(i, j, m)G_{ m, h}(a, j) W_h(s, i)\\
    &= \Tilde W'_h(s){G}_h(a)^\top
\end{align*}
and $P(s'|\cdot, \cdot) = \Tilde{G}_h U'_h(s')^\top$ (with the same argument) for some $\cardS \times dM$ matrices $W'_h, U_h'(s')$ with entries bounded by $\alpha$. Note that $W'_h$ and $U_h'(s')$ are matrices that join $W_{m, h}$ and $U_{m, h}(s')$, respectively, with entries that at most $\alpha$ times larger than the original entry. 
 
Therefore, it follows for all $(s', s, a, h) \in \cS\times \cS\times \cA\times [H]$, 
\begin{align*}
 |r_h(s, a)  - \hat{\Tilde{G}}_h(a)R_hW'_h(s)^\top | &= |\Tilde{G}_h(a)W'_h( s)^\top  - \hat{\Tilde{G}}_h(a)R_hW'_h(s)^\top| \\
&=  |(\Tilde{G}_{h}(a) -\hat{\Tilde{G}}_h(a) R_h)W'_h(s) | \\
&= \alpha | \sum_{m \in M}(G_{m, h}(a) -  \hat{G}_{m, h}(a)R_{m, h}) W_{m, h}(s)|\\
&\leq \alpha \sum_{m \in M} \|G_{m, h}(s) -  \hat{G}_{m, h}(s)R_{m, h} \|_2 \|W_{m, h}(s) \|_2\\
&\leq \alpha \sqrt{\frac{\cardA }{d\mu}} \sum_{m \in M} \|G_{m, h}(a) -  \hat{G}_{m, h}(a)R_{m, h} \|_2 \\
&\leq \sqrt{\frac{dHM\cardS }{T}}
\end{align*}
from the Cauchy-Schwarz inequality and our singular vector perturbation bound. From the same logic,
\begin{align*}
\|P_h(\cdot|s, a)  - \hat{\Tilde{G}}_h(a)R_h U'_h(s', s)^\top \|_{TV} &\leq |\sum_{s' \in S} P_h(s'|s, a)  - \hat{\Tilde{G}}_h(a)R_h U'_h(s', s)^\top |\\
&= |\sum_{s' \in S} \Tilde{G}_h(a)U'_h(s', s)  -\hat{\Tilde{G}}_h(a)R_h U'_h(s', s)^\top |\\
&\leq \alpha | \sum_{m \in M}(G_{m, h}(a) -  \hat{G}_{m, h}(a)R_{m, h}) \sum_{s' \in S} U_{m,h}(s', s)|\\
&\leq \alpha \sum_{m \in M} \|(G_{m, h}(a) -  \hat{G}_{m, h}(a)R_{m, h}) \|_2 \|\sum_{s' \in S} U_{m, h}(s', s)^\top\|_2\\
&\leq \sqrt{\frac{d H M \cardA }{T}}.
\end{align*}

Therefore, $\hat{\Tilde{G}}_h(s)$ satisfies Assumption \ref{asm:miss_s} with $\xi = \sqrt{\frac{dMH \cardS }{T }}$. Then it follows that running LSVI-UCB-TR using $\hat{\Tilde{G}}_h(a)$  with $\delta' = \delta /2$ during the target phase of the algorithm admits a regret bound of 
\[
Regret(T) \leq C" (\sqrt{d^3M^3H^3\cardS T} + dMHT\sqrt{\frac{dMH \cardS }{T }}) \in \Tilde{O}(\sqrt{d^3M^3H^3\cardS T})
\]
with probability at least $1 - \delta$ from a final union bound. Furthermore, the sample complexity in the source phase is 
\[
\Tilde{O} \left( \frac{d^5 \mu^4\kappa^4(\cardS +\cardA )M^2  H^4\alpha^2  T}{\cardS } \right), 
\]
which proves our result.    
\end{proof}
